# Supplementary material for: FlexOS: Towards Flexible OS Isolation
Source: arXiv:2112.06566 source file (2022-01-14)
Supplement: Supplementary file 1 [file appendix.tex]

\appendix
\section{\lang specification}
\label{appendix:a}
% the \\ insures the section title is centered below the phrase: AppendixA
 A detailed overview of the \lang
specification syntax is below:

\begin{scriptsize}
\begin{Verbatim}[commandchars=\#+!]
<#userinput+[Memory Access]!> ::= <access modifier>? {<memory model>}
<#userinput+[Call]!> ::=  <execution modifier>? {<execution model>}
<#userinput+[API]!> ::=  {<execution model>}
<#userinput+[Requires]!> ::= <access modifier>? {<memory model>} | \
                  {<execution modifier>? \
                  {<execution model>}}
  <memory model> :: = (#userinput+<ptr>!, <basic access modifier>, \
                       #userinput+<size>!, #userinput+<memtype>!)
  <access modifier> ::== <basic access modifier>|#userinput+R*!|#userinput+W*!|#userinput+U!
  <basic access modifier> ::= #userinput+R!|#userinput+W!
  <execution modifier> ::= #userinput+U!|#userinput+X!|#userinput+X*!
  <execution model> ::= (#userinput+<ptr>!, #userinput+<call type>!)
\end{Verbatim}
\end{scriptsize}

We use \texttt{\{\}} to mark repetition, \texttt{?} for optional terms
and bold to mark terminals.

\texttt{[Memory Access]} specifies memory access properties for the
component. \textit{R/W} grants read/write access to shared memory,
\textit{R*/W*} grants read/write access to all the memory.  For a more
fine-grained specification, the tuple \textit{(<ptr>, <basic access
  modifier>, <size>, <memtype>)} can be used to enact read/write
properties for a \textit{memtype} element.  A \textit{memtype} element
can be a memory address or segment.

\texttt{[Call]} adds properties for calls to outer components. We have
a coarse grained specification: \textit{U} means no call, \textit{X}
will respect the control flow, and \textit{X*} means that the
component may jump-access anywhere in outer components without
constraints (e.g. it may change the stack return address through a
buffer overflow). The fine-grained specification uses a tuple to
specify symbols or addresses where the component may
jump-access. \textit{call type} can be either \textit{SYMB} for a
symbol or \textit{ADDR} for an address.  Note that both
\texttt{<Memory Access>} and \texttt{<Call>} should be used to
describe the component's behavior under normal but also adversarial
operation: a component written in a memory unsafe language with no
particular level of verification should be marked as able to
read/write/jump anywhere in memory.

\texttt{[API]} is used to register the API provided to other
components. Both symbols and addresses may be specified. The exported
symbols may be later used in the specification of other
components. They are meant to be used by components that are closely
related.

\texttt{[Requires]} specifies preconditions for outer components. It
encapsulates both \texttt{[Memory Access]} and \texttt{[Call]} maximum
properties that outer components must have when calling the current
component in the same compartment.
